# Supplementary material for: ReManNet: A Riemannian Manifold Network for Monocular 3D Lane Detection
Source: arXiv:2603.19776 source file (2026-03-20)
Supplement: Supplementary file 1 [file X_suppl.tex]

\clearpage
\setcounter{page}{1}
\maketitlesupplementary

\newtheorem{lemma}{Lemma}[section]
\newtheorem{theorem}{Theorem}[section]
\newtheorem{proof}{Proof}[section]

\newcommand{\norm}[1]{\left\lVert#1\right\rVert}
\newcommand{\R}{\mathbb{R}}
\newcommand{\pd}[2]{\frac{\partial#1}{\partial#2}}
\newcommand{\dd}[2]{\frac{\mathrm{d}#1}{\mathrm{d}#2}}

\appendix

\begin{center}
\section*{Overview}
\end{center}

\noindent This supplementary material is organized as follows:
\begin{itemize}
    \item Section~\ref{app:road_manifold} presents the geometric foundations of the Road-Manifold Assumption, from design axioms to a formal proposition.
    \item Section~\ref{app:qualitative} presents qualitative visualizations of 3D lane predictions and a detailed runtime–accuracy analysis.
    \item Section~\ref{app:openlane_ablation} presents ablation studies on the OpenLane dataset, examining the effect of the ReManNet components and the proposed 3D-TIoU loss.
\end{itemize}

\section{Road-Manifold Assumption: Geometric Foundations}
\label{app:road_manifold}

Lacking an invariant geometric--topological coupling between lanes and the
underlying road surface, 2D-to-3D lifting is ill-posed and brittle, often
degenerating into concavities, bulges, and twists as illustrated in
Fig.~\ref{fig:failure-modes}. Small perturbations in image-space lane
predictions can lead to large and physically implausible deformations of the
induced 3D road surface.

\begin{figure}[htbp]
  \centering
  \begin{subfigure}{0.32\linewidth}
    \centering
    \includegraphics[width=\linewidth]{concavities.png}
    \caption{Concavity.}
    \label{fig:concavity}
  \end{subfigure}
  \hfill
  \begin{subfigure}{0.32\linewidth}
    \centering
    \includegraphics[width=\linewidth]{bulges.png}
    \caption{Bulge.}
    \label{fig:bulge}
  \end{subfigure}
  \hfill
  \begin{subfigure}{0.32\linewidth}
    \centering
    \includegraphics[width=\linewidth]{twists.png}
    \caption{Twist.}
    \label{fig:twist}
  \end{subfigure}
  \caption{Failure modes of 2D-to-3D lifting without geometric--topological
  structure. When the coupling between lanes and the underlying road surface
  is not explicitly modeled, the reconstructed geometry can easily degenerate
  into concavities, bulges, and twisted surfaces, even when the 2D lane
  projections look plausible.}
  \label{fig:failure-modes}
\end{figure}

To address this, we propose the \emph{Road-Manifold Assumption}: the road
surface is modeled as a smooth two-dimensional manifold $\mathcal{M}\subset
\R^3$, lane centerlines are embedded one-dimensional submanifolds
$\gamma_j\subset\mathcal{M}$, and sampled lane points are dense observations
on these curves. This construction couples metric and topology across the
surface, the lane curves, and their discrete samples, providing a stable
geometric space for 2D-to-3D lifting.
\subsection{Geometric Design Axioms}
\label{app:axioms}

According to Wolhuter's \emph{Geometric Design of Roads Handbook}~\cite{wolhuter2015geometricroaddesign1} and and common engineering sense,
geometric design requires continuity of alignment,
gradual variation of curvature, and smooth grade transition.
Formally, let
\begin{equation}
    \bm{c}(s) = \big(x(s),y(s),z(s)\big)^\top \in \R^3
\end{equation}
denote the spatial trajectory of the road centerline parameterized by station
coordinate $s$. We assume
\begin{equation}
    x,y,z \in C^2(I),
\end{equation}
for some interval $I \subset \R$.

\noindent\textbf{Horizontal curvature.}
The plan-view centerline is
\begin{equation}
    \bm{p}(s) = \big(x(s),y(s)\big)^\top,
\end{equation}
with horizontal curvature
\begin{equation}
    \kappa_h(s)
    =
    \frac{|x'(s)y''(s)-y'(s)x''(s)|}
         {\big(x'(s)^2+y'(s)^2\big)^{3/2}}.
    \label{eq:kappa_h}
\end{equation}
Design constraints~\cite{wolhuter2015geometricroaddesign1} impose a minimum radius
$R_{\min}(V)$ and bounded rate of curvature change for design speed $V$, which we
encode as
\begin{equation}
\label{eq:kappa_bound}
\begin{gathered}
    0 \leq \kappa_h(s) \leq \kappa_{h,\max}(V), \\
    \kappa_{h,\max}(V) \triangleq \frac{1}{R_{\min}(V)}, \\
    |\kappa_h'(s)| \leq \alpha_{\max}(V) < \infty.
\end{gathered}
\end{equation}

This formalizes ``gradual variation of curvature'' and excludes broken-back
curves and sharp kinks.

\noindent\textbf{Vertical grade and $K$-values.}
The vertical profile follows a parabolic curve~\cite[Ch.~7]{wolhuter2015geometricroaddesign1}:
\begin{equation}
\label{eq:vertical_parabola}
\begin{gathered}
    z(s) = a s^2 + b s + c, \\
    g(s) \triangleq \dd{z}{s} = 2 a s + b, \\
    \dd{g}{s} = 2a = \text{constant}.
\end{gathered}
\end{equation}

In standard notation, for a vertical curve of length $L$ connecting grades
$g_1$ and $g_2$ with grade difference $A = g_2-g_1$, the $K$-value is
\begin{equation}
    K \triangleq \frac{L}{A},
    \qquad
    \frac{\mathrm{d}^2 z}{\mathrm{d}s^2}
    =
    \frac{A}{L}
    =
    \frac{1}{K}.
\end{equation}
Sight-distance and comfort limits yield a minimum $K_{\min}(V)$, and
\begin{equation}
    K \geq K_{\min}(V)
    \;\Longleftrightarrow\;
    \Big|\frac{\mathrm{d}^2 z}{\mathrm{d}s^2}\Big|
    \leq \frac{1}{K_{\min}(V)}.
    \label{eq:K_bound}
\end{equation}
Thus $z \in C^2(I)$ with bounded second derivative.

\noindent\textbf{Spatial curvature and grade bounds.}
The full spatial curvature of $\bm{c}(s)$ is
\begin{equation}
    \kappa(s)
    =
    \frac{\norm{\bm{c}'(s) \times \bm{c}''(s)}}
         {\norm{\bm{c}'(s)}^3},
    \label{eq:kappa_3d}
\end{equation}
which depends on both horizontal and vertical alignment. Combining
\eqref{eq:kappa_bound}, \eqref{eq:vertical_parabola}, and \eqref{eq:K_bound},
geometric design yields global bounds
\begin{equation}
\label{eq:kappa_grade_bounds}
\begin{gathered}
    |\kappa(s)| \leq \kappa_{\max}, \\
    |g(s)| \leq g_{\max}, \\
    |\kappa'(s)| < \infty,\quad |g'(s)| < \infty.
\end{gathered}
\end{equation}

These constraints define a smooth, nonsingular centerline used in design
consistency~\cite[\S4.5]{wolhuter2015geometricroaddesign1}.

\subsection{Surface Definition and Regularity}
\label{sec:surface_app}

We model the road surface as a parametric mapping
\begin{equation}
    F(u,v) =
    \begin{bmatrix}
        x(u,v)\\[2pt]
        y(u,v)\\[2pt]
        z(u,v)
    \end{bmatrix},
    \qquad (u,v)\in \mathcal{U} \subset \R^2,
    \label{eq:surface_param}
\end{equation}
where $u$ represents longitudinal stationing and $v$ the lateral offset.
A standard choice consistent with road coordinates is
\begin{equation}
    F(u,v)
    =
    \bm{c}(u)
    + v\,\bm{n}(u)
    + h(u,v)\,\bm{e}_z,
\end{equation}
where $\bm{c}(u)$ is the centerline from \eqref{eq:vertical_parabola},
$\bm{n}(u)$ is a lateral unit vector orthogonal to the tangent
$\bm{c}'(u)$ in the horizontal plane, $h(u,v)$ is the elevation
contribution of crossfall and superelevation, and
\begin{equation}
    \bm{e}_z = (0,0,1)^\top
\end{equation}
is the global vertical unit vector.

The Jacobian
\begin{equation}
    J(u,v)
    =
    \big[F_u(u,v)\;\;F_v(u,v)\big]
    =
    \big[\pd{F(u,v)}{u}\;\; \pd{F(u,v)}{v}\big]
\end{equation}
is assumed to satisfy
\begin{equation}
    \operatorname{rank}(J(u,v)) = 2,
    \qquad \forall (u,v)\in \mathcal{U},
    \label{eq:rank2}
\end{equation}
reflecting Wolhuter's ``nonsingular geometry and gradual curvature variation''.
Under \eqref{eq:kappa_grade_bounds} and smooth crossfall variation, \eqref{eq:rank2} holds.
Hence the image
\begin{equation}
    \mathcal{M} = F(\mathcal{U})\subset\R^3
\end{equation}
is a regular embedded two-dimensional submanifold.
\begin{lemma}[Smooth road surface]
\label{lem:road_surface_app}
If $x,y,z\in C^2$ satisfy~\eqref{eq:kappa_grade_bounds}, and
$\operatorname{rank}(J(u,v)) = 2$ for all $(u,v)\in\mathcal{U}$, then
$\mathcal{M} = F(\mathcal{U})$ is a $C^2$ embedded surface in
$\R^3$.
\end{lemma}
\subsection{Induced Riemannian Structure}
\label{sec:riemann_app}

The metric tensor $g$ on $\mathcal{M}$ is induced from the Euclidean inner
product $\langle\cdot,\cdot\rangle$:
\begin{equation}
    g_{ij}(u,v)
    = 
    \left\langle
        \pd{F}{u_i}(u,v),
        \pd{F}{u_j}(u,v)
    \right\rangle,
    \quad
    (u_1,u_2)\equiv(u,v).
\end{equation}
Writing
\begin{equation}
    E = \langle F_u,F_u\rangle,\quad
    F = \langle F_u,F_v\rangle,\quad
    G = \langle F_v,F_v\rangle,
\end{equation}
we obtain the first fundamental form
\begin{equation}
    g(u,v)
    =
    \begin{pmatrix}
        E & F\\
        F & G
    \end{pmatrix},
    \qquad
    EG-F^2 > 0,
    \quad E,G>0.
\end{equation}
The condition $EG-F^2>0$ is equivalent to
\begin{equation}
    \det g(u,v)
    =
    \norm{F_u(u,v)\times F_v(u,v)}^2 > 0,
\end{equation}
so $g$ is positive definite and $(\mathcal{M},g)$ is Riemannian.
The intrinsic arc-length between two points $p,q\in\mathcal{M}$ is
\begin{equation}
    d_g(p,q)=
    \inf_{\gamma}
    \int_{0}^{1}
    \sqrt{g_{\gamma(t)}(\dot{\gamma}(t),\dot{\gamma}(t))}\,\mathrm{d}t,
\end{equation}
where $\gamma:[0,1]\to\mathcal{M}$ is any smooth curve joining them.

\subsection{Lane Curves as One-Dimensional Submanifolds}
\label{sec:lanes_submanifold_app}

Each lane centerline is modeled as a one-dimensional $C^2$ embedded
submanifold of $\mathcal{M}$:
\begin{equation}
    \gamma_j:I_j\to\mathcal{M},\quad
    \gamma_j(\tau) = \big(x_j(\tau),y_j(\tau),z_j(\tau)\big)^\top,
\end{equation}
with non-vanishing tangent
\begin{equation}
    \norm{\dot{\gamma}_j(\tau)}_g>0,
    \qquad \forall \tau\in I_j.
\end{equation}
The geodesic curvature is
\begin{equation}
    \kappa_j(\tau) = \norm{\nabla_{\dot{\gamma}_j}\dot{\gamma}_j}_g,
\end{equation}
where $\nabla$ is the Levi-Civita connection associated with $g$.

From the geometric consistency principle~\cite[\S4.5]{wolhuter2015geometricroaddesign1}
and side-friction/superelevation limits, we have approximately constant curvature rate
and explicit bounds
\begin{equation}
\label{eq:lane_bounds}
\begin{gathered}
    \dd{\kappa_j}{\tau} \approx 0, \\[2pt]
    |\kappa_j(\tau)| \le 
    \frac{\tan(e_{\max}) + f_{\max}}{V_j^2 / 127}, \\[2pt]
    |g_j(\tau)| \le g_{\max}.
\end{gathered}
\end{equation}

\begin{lemma}[Lane regularity]
\label{lem:lane_regular_app}
If $\gamma_j \in C^2(I_j)$, $\dot{\gamma}_j\neq 0$, and
$\gamma_j(\tau)\in\mathcal{M}$ for all $\tau$, then the image of $\gamma_j$
is a one-dimensional embedded submanifold of $\mathcal{M}$.
\end{lemma}

\begin{figure*}[t]
    \centering
    % 需要 \usepackage{array}
    \setlength{\tabcolsep}{10pt}   % horizontal spacing between columns

    % R 列：窄一点，用来放行号；I 列：放图片
    \newcolumntype{R}{>{\centering\arraybackslash}m{0.03\textwidth}}
    \newcolumntype{I}{>{\centering\arraybackslash}m{0.30\textwidth}}

    \begin{tabular}{R@{\hspace{8pt}}I@{\hspace{8pt}}I@{\hspace{10pt}}I}
        & \textbf{Anchor3d (Baseline)} &
          \textbf{Anchor3d++ (SOTA)} &
          \textbf{ReManNet (Ours)} \\[10pt]

        \textbf{1} &
        \includegraphics[width=\linewidth]{anchor1.png} &
        \includegraphics[width=\linewidth]{anchor++1.png} &
        \includegraphics[width=\linewidth]{spd1.png} \\[10pt]

        \textbf{2} &
        \includegraphics[width=\linewidth]{anchor2.png} &
        \includegraphics[width=\linewidth]{anchor++2.png} &
        \includegraphics[width=\linewidth]{spd2.png} \\[10pt]

        \textbf{3} &
        \includegraphics[width=\linewidth]{anchor3.png} &
        \includegraphics[width=\linewidth]{anchor++3.png} &
        \includegraphics[width=\linewidth]{spd3.png} \\[10pt]

        \textbf{4} &
        \includegraphics[width=\linewidth]{anchor4.png} &
        \includegraphics[width=\linewidth]{anchor++4.png} &
        \includegraphics[width=\linewidth]{spd4.png} \\
    \end{tabular}
    \caption{Qualitative evaluation results on OpenLane. The scenarios include daytime, nighttime, curved roads, multi-lane scenes, shadows, and occlusions. Ground-truth lanes are shown as red lines, while lines in other colors denote predictions; different colors correspond to different lane-marking categories.}
    \label{fig:qual_openlane}
\end{figure*}

\subsection{Discretization Consistency with 3D Lane Representation}
\label{sec:discrete_consistency_app}

A 3D lane representation~\cite{chen2022persformerbev1,guo2020genbev3} is
\begin{equation}
    \bm{L}_j=(\bm{P}_j,C_j),
    \qquad 
    \bm{P}_j=
    \big\{(x_i^j,y_i^j,z_i^j)\big\}_{i=1}^{Q},
\end{equation}
with fixed longitudinal coordinates $Y_{\text{ref}}=\{y_i\}$.
Assuming samples lie on $\gamma_j$, we have
\begin{equation}
    (x_i^j,y_i^j,z_i^j) = \gamma_j(y_i^j),
    \qquad y_i^j \in Y_{\text{ref}}.
\end{equation}
High sampling density in the intrinsic metric $g$ implies
\begin{equation}
    \max_i d_g\big(\gamma_j(y_i^j),\gamma_j(y_{i+1}^j)\big) < \varepsilon
    \;\Longrightarrow\;
    \lim_{\varepsilon\to0}\bm{P}_j\to\gamma_j
    \text{ in }C^1.
\end{equation}
Hence discrete lanes approximate smooth submanifolds on $\mathcal{M}$.

\subsection{Verification of Road-Manifold Conditions}
\label{sec:verification_app}

\noindent\textbf{(1) Local homeomorphism.}
Alignment continuity and the rank condition~\eqref{eq:rank2} provide
local charts $(\mathcal{U}_\alpha,\varphi_\alpha)$ covering $\mathcal{M}$.

\noindent\textbf{(2) Smooth transition maps.}
At tangent junctions and grade transitions, $C^1$ continuity of
curvature and grade ensure $C^\infty$ chart transitions
$\varphi_\beta\circ\varphi_\alpha^{-1}$ on overlaps
$\mathcal{U}_\alpha\cap\mathcal{U}_\beta$. Let
\begin{equation}
    \mathcal{G} = \{(\mathcal{U}_\alpha,\varphi_\alpha)\}
\end{equation}
denote the induced atlas.

\noindent\textbf{(3) Consistency of curvature and grade.}
Bounded $\kappa_h'(s)$ and $g'(s)$ imply at least $C^2$ smoothness of
the centerline and surface fields, and exclude abrupt changes in
alignment and grade. For our purposes, it is sufficient to assume that
there exist tolerances $\tau,\eta>0$ such that
\begin{equation}
    \bigl|\dd{g}{s}\bigr| < \tau,
    \qquad 
    \bigl|\dd{\kappa}{s}\bigr| < \eta,
\end{equation}
which enforces the gradual variation of vertical grade and spatial curvature
along the road.

\begin{table}[t]
    \centering
    \small
    \setlength{\tabcolsep}{6pt}  % 调整列间距，可根据版面再微调
    \begin{tabular}{l|c|c}
        \toprule
        \textbf{Method} & \textbf{F1 (\%) $\uparrow$} & \textbf{FPS$\uparrow$} \\
        \midrule
        3D-LaneNet~\cite{garnett20193dbev2} \scriptsize{[CVPR'19]}        & 44.1 & 67.5 \\
        GenLaneNet~\cite{guo2020genbev3} \scriptsize{[ECCV'20]}           & 32.3 & 16.6 \\
        PersFormer~\cite{chen2022persformerbev1} \scriptsize{[ECCV'22]}   & 50.5 & 18.1 \\
        MapTRv2 (R50)~\cite{liao2025maptrv2} \scriptsize{[ICRA'23]}       & 53.6 & 26.0 \\
        LATR-Lite~\cite{luo2023latr} \scriptsize{[ICCV'23]}               & 61.5 & 23.5 \\
        LATR~\cite{luo2023latr} \scriptsize{[ICCV'23]}                    & 61.9 & 15.2 \\
        Anchor3DLane (R18)~\cite{huang2023anchor3dlaneanchor1} \scriptsize{[CVPR'23]}           & 53.7 & \textbf{72.1} \\
        Anchor3DLane (R50)$^\dagger$~\cite{huang2023anchor3dlaneanchor1} 
            \scriptsize{[CVPR'23]}                                        & 57.5 & 32.7 \\
        Anchor3DLane++ (R18)~\cite{huang2024anchor3dlane++anchor2} 
            \scriptsize{[TPAMI'24]}                                       & 57.9 & 38.1 \\
        Anchor3DLane++ (R50)~\cite{huang2024anchor3dlane++anchor2} 
            \scriptsize{[TPAMI'24]}                                       & 62.4 & 22.9 \\           
        Glan3D (R18)~\cite{ozturk2025glane3dbev5key2} \scriptsize{[CVPR'25]} 
                                                                          & 61.5 & 62.2 \\
        Glan3D (R50)~\cite{ozturk2025glane3dbev5key2} \scriptsize{[CVPR'25]} 
                                                                          & 63.9 & 27.8 \\
        \rowcolor{gray!12}
        ReManNet (R18) (Ours)                                             & 63.5 & 53.2 \\
        \rowcolor{gray!12}
        ReManNet (R50) (Ours)                                             & \textbf{65.7} & 26.7 \\
        \bottomrule
    \end{tabular}
    \caption{
        Comparison of model performance in terms of F1 score and inference speed (FPS).
        R18 and R50 denote ResNet-18 and ResNet-50 backbones, respectively; 
        $^\dagger$ marks the baseline model. The best results are highlighted in bold.
    }
    \label{tab:3dlane_results}
\end{table}

\begin{table}[t]
  \centering
  \footnotesize
  \setlength{\tabcolsep}{4.5pt}
  
  \begin{tabular}{c c c | c}
    \toprule
    \textbf{Baseline} & 
    \makecell[c]{\textbf{Riemannian manifold}\\\textbf{embedding layer}} & 
    \makecell[c]{\textbf{Gated Feature}\\\textbf{Fusion Layer}} &
    \textbf{F1 (\%)} $\uparrow$ \\
    \midrule
    \checkmark &  &  & 57.5 \\
    \checkmark & \checkmark &  & 21.8 \\
    \checkmark & \checkmark & \checkmark & \textbf{65.7} \\
    \bottomrule
  \end{tabular}
  \caption{Additional ablation study of ReManNet components on the OpenLane validation set.}
  \label{tab:ablation_Components}
\end{table}

\subsection{Formal Proposition and Proof Outline}
\label{sec:formal_prop_app}

\begin{theorem}[Road-Manifold realization]
\label{thm:road_manifold_realization}
Under Wolhuter's geometric continuity axioms (Sec.~\ref{app:axioms}) and the
curvature/grade bounds in~\eqref{eq:kappa_grade_bounds}, the triplet
$(\mathcal{M},\mathcal{G},g)$, where $\mathcal{G}$ is the atlas induced by
$F$ and $g$ is the pullback metric, constitutes a globally smooth $C^2$
Riemannian submanifold of $\R^3$. Moreover, each lane
$\gamma_j\subset\mathcal{M}$ is a regular one-dimensional embedded
submanifold.
\end{theorem}

\begin{proof}[Sketch]
Lemma~\ref{lem:road_surface_app} together with the rank condition~\eqref{eq:rank2}
implies that $F$ is a $C^2$ immersion and $\mathcal{M}=F(\mathcal{U})$ is an
embedded surface. The positivity of the first fundamental form yields a
Riemannian metric $g$ on $\mathcal{M}$. Finally,
Lemma~\ref{lem:lane_regular_app} guarantees that each lane curve $\gamma_j$
is a regular one-dimensional embedded submanifold of $\mathcal{M}$, which
establishes the stated road-manifold structure.
\end{proof}

\section{Qualitative Evaluation and Efficiency Analysis}
\label{app:qualitative}
\subsection{Qualitative Evaluation}
As shown in Fig.~\ref{fig:qual_openlane}, the qualitative evaluation indicates that our method achieves more accurate lane recognition and localization than both the baseline Anchor3d \cite{huang2023anchor3dlaneanchor1} and the Anchor3d++ \cite{huang2024anchor3dlane++anchor2} SOTA counterpart. In particular, under challenging nighttime conditions with limited illumination, our approach produces noticeably fewer missed and misplaced lanes, highlighting its robustness to low-visibility scenarios. These improvements suggest that the proposed Riemannian manifold modeling of lane geometry provides a more reliable representation for 3D lane detection across diverse scenes.

\subsection{Runtime and Accuracy Analysis}
\label{subsec:runtime_accuracy}

As shown in Table~\ref{tab:3dlane_results}, ReManNet achieves a favorable trade-off between accuracy and efficiency compared with existing 3D lane detection methods~\cite{garnett20193dbev2,guo2020genbev3,chen2022persformerbev1,liao2025maptrv2,luo2023latr,huang2023anchor3dlaneanchor1,huang2024anchor3dlane++anchor2,ozturk2025glane3dbev5key2}. 
With a ResNet-50 backbone, ReManNet attains the highest F1 score of \textbf{65.7}, outperforming prior transformer-based approaches such as LATR (61.9) and LATR-Lite (61.5)~\cite{luo2023latr}, as well as the recent Glan3D (R50) (63.9)~\cite{ozturk2025glane3dbev5key2}. 
Compared with the baseline Anchor3DLane (R50)$^\dagger$ (57.5 F1, 32.7 FPS)~\cite{huang2023anchor3dlaneanchor1}, ReManNet (R50) improves the F1 score by \textbf{8.2} points while maintaining a comparable inference speed (26.7 FPS), indicating that the performance gain does not come at a significant runtime cost.
Meanwhile, its inference speed of 26.7 FPS is comparable to MapTRv2 (R50) (26.0 FPS)~\cite{liao2025maptrv2} and Glan3D (R50) (27.8 FPS)~\cite{ozturk2025glane3dbev5key2}.

The lightweight ReManNet (R18) further demonstrates the scalability of our design. 
It achieves an F1 score of \textbf{63.5}, surpassing Anchor3DLane++ (R50) (62.4)~\cite{huang2024anchor3dlane++anchor2} and Glan3D (R18) (61.5)~\cite{ozturk2025glane3dbev5key2}, while running at 53.2 FPS, which is substantially faster than most high-accuracy baselines, such as LATR (15.2 FPS) and LATR-Lite (23.5 FPS)~\cite{luo2023latr}. 
Although Anchor3DLane (R18)~\cite{huang2023anchor3dlaneanchor1} attains the highest throughput (72.1 FPS), it lags far behind in accuracy (53.7 F1). 
These results validate that ReManNet consistently offers a superior accuracy--efficiency trade-off across different backbone capacities.

\begin{figure}[t]
  \centering
  \begin{subfigure}{\linewidth}
    \centering
    \includegraphics[width=0.8\linewidth]{3D-TLIOUv2.png}
    \caption{2D illustration on the slice $Y = Y_i$.}
    \label{fig:3dtliou-2d}
  \end{subfigure}
  \vspace{0.3em}
  \begin{subfigure}{\linewidth}
    \centering
    \includegraphics[width=0.8\linewidth]{3d-tube.png}
    \caption{3D illustration of the tubular intersection.}
    \label{fig:3dtliou-3d}
  \end{subfigure}
  \caption{%
  2D \textbf{(a)} and 3D \textbf{(b)} illustration of the proposed 3D-TLIoU loss.
  The red point $\mathbf{p}_i$ and green point $\mathbf{g}_i$ denote the predicted
  and ground-truth 3D lane points, respectively. 
  Each point is expanded into a tube of radius $r_{\text{tube}}$ in 3D space.
  The overlap term $d_{\text{over}}$ measures how much the two tubes overlap
  along the line connecting $\mathbf{p}_i$ and $\mathbf{g}_i$, and is defined as
  $d_{\text{over}} = 2 r_{\text{tube}} - \|\mathbf{p}_i - \mathbf{g}_i\|$.
  It can be negative when the tubes are separated, indicating how far apart
  the two points are (blue arrows).
  The union term $d_{\text{union}}$ is the extent of the union along the same line,
  given by $d_{\text{union}} = 2 r_{\text{tube}} + \|\mathbf{p}_i - \mathbf{g}_i\|$
  (purple arrows).%
  }
  \label{fig:3dtliou}
\end{figure}

\section{Additional Ablation Studies}
\label{app:openlane_ablation}

\subsection{ReManNet components.} To better understand the role of the manifold embedding and the gating
mechanism, we further consider a \emph{geometry-only} variant that removes
both the gate and the visual features. Concretely, starting from the
Riemannian manifold embedding layer, which produces a global
Riemannian Gaussian descriptor $\mathbf{H}\in\mathbb{R}^{B\times d_h}$ for
each sample, we expand $\mathbf{H}$ over anchors,
\begin{equation}
    \widetilde{\mathbf{H}}=\operatorname{expand}(\mathbf{H})
    \in\mathbb{R}^{B\times A\times d_h},
\end{equation}
and directly feed it into a per-anchor prediction head:
\begin{equation}
    \mathbf{F}_{\mathrm{geo}}
    =
    \phi(\widetilde{\mathbf{H}})
    \in\mathbb{R}^{B\times A\times d_h},
\end{equation}
where $\phi(\cdot)$ is a shared linear (or shallow MLP) transformation applied
independently to each anchor. The classification and regression heads then
operate on $\mathbf{F}_{\mathrm{geo}}$, without any contribution from
$\mathbf{F}_{\mathrm{anchor}}$ or the gate $\mathbf{g}$.

We compare three configurations on the OpenLane validation set:
(i) the Anchor3d baseline \cite{huang2023anchor3dlaneanchor1},
(ii) the geometry-only variant described above, and
(iii) the full ReManNet with gated fusion. Results are summarized in
Table~\ref{tab:ablation_Components}.

Starting from the Anchor3d  baseline (Row~1), we then examine the
geometry-only variant in Row~2. In this configuration, the Riemannian
manifold embedding layer is used as the \emph{only} source of features for
the second-stage prediction: both the gate and the visual anchor features
are removed, and the classifier and regressor operate solely on the
Riemannian Gaussian descriptor $\widetilde{\mathbf{H}}$. This design leads
to a pronounced degradation, with F1 dropping from $57.5\%$ to $21.8\%$.
It indicates that a global manifold statistical operator by itself is too
coarse to capture fine-grained, anchor-level appearance and localization
cues, and thus cannot serve as a reliable standalone representation for 3D
lane detection. 

From a broader perspective, this observation is consistent
with the empirical role of $\mathrm{Sym}_+^n$ layers in neural networks:
SPD embeddings are particularly well-suited to encode global, invariant
statistics for recognition or classification \cite{nguyen2021geomnetspd1action1, zhang2020deepspdaction2, sun2017learningscenerego1, wang2021symnetscenerego2, brooks2019riemannianface1, huang2017riemannianface2}, but the very pooling and
aggregation operations that make them robust also tend to wash out
fine-grained spatial correspondences that are critical for precise
geometric regression. In other words, using $\mathrm{Sym}_+^n$ features
without any anchor-aware conditioning effectively decouples the manifold
descriptor from the underlying pixel- and anchor-level geometry, which
explains the limited performance of the geometry-only variant in this
regression-heavy 3D lane detection setting.

In contrast, when we introduce the proposed gated visual--geometric fusion
layer (Row~3), the manifold embedding is no longer used as an isolated
predictor, but as a residual correction on top of the anchor-wise visual
features. This design not only recovers the performance loss of the
geometry-only variant, but also substantially surpasses the original baseline,
boosting F1 from $57.5\%$ to $65.7\%$. Taken together, these ablations indicate
that (i) the Riemannian manifold embedding layer must be coupled with
anchor-level visual evidence to provide useful, fine-grained supervision, and
(ii) the gating mechanism is critical for selectively injecting manifold
geometry, so that ReManNet can exploit the global statistical structure of
3D lanes without undermining the fidelity of local regression, thereby
substantially improving overall detection accuracy.

\subsection{3D-TLIoU Loss.} 
\label{subsec:3d_tliou}

\begin{table}[t]
    \centering
    \small
    \setlength{\tabcolsep}{8pt} % 可根据版面微调
    \begin{tabular}{cc}
        \toprule
        $\mathbf{r_\text{tube}}$ & \textbf{F1 (\%)$\uparrow$} \\
        \midrule
        0.5 & 64.59 \\
        1.0 & 65.08 \\ % 若有结果可填上
        1.5 & \textbf{65.74} \\
        2.0 & 65.73 \\
        2.5 & 65.58 \\
        \bottomrule
    \end{tabular}
    \caption{Effect of the tube radius $r_\text{tube}$ on 3D lane detection performance on OpenLane (ReManNet-R50).}
    \label{tab:tube_radius}
\end{table}

As illustrated in Fig.~\ref{fig:3dtliou}, the proposed 3D-TLIoU loss lifts the point-wise discrepancy between predicted and ground-truth 3D lane points into a tubular intersection measure. 
Each 3D point $\mathbf{p}_i$ and $\mathbf{g}_i$ is expanded into a tube of radius $r_\text{tube}$, and the loss is computed from the overlap term $d_{\text{over}} = 2 r_{\text{tube}} - \|\mathbf{p}_i - \mathbf{g}_i\|$ and the union term $d_{\text{union}} = 2 r_{\text{tube}} + \|\mathbf{p}_i - \mathbf{g}_i\|$ along the line connecting $\mathbf{p}_i$ and $\mathbf{g}_i$. 
When the tubes intersect ($d_{\text{over}} > 0$), the loss focuses on how well the two local lane tubes align, whereas for separated tubes ($d_{\text{over}} < 0$), it behaves as a distance-aware penalty that quantifies how far the prediction deviates from the ground truth.

Table~\ref{tab:tube_radius} reports an ablation study on the tube radius $r_\text{tube}$ for ReManNet-R50 on the OpenLane dataset. 
The performance is relatively stable for $r_\text{tube} \in [1.0, 2.5]$, with F1 scores ranging from 65.08\% to 65.74\%, indicating that the 3D-TLIoU loss is not overly sensitive to the exact choice of radius. 
A small radius (e.g., $r_\text{tube}=0.5$) leads to a noticeable drop to 64.59\% F1, suggesting that an overly tight tube makes the loss behave similarly to a hard point-wise distance, reducing its tolerance to minor localization noise. 
The best performance is achieved at $r_\text{tube}=1.5$ (65.74\% F1), slightly outperforming larger radii such as $r_\text{tube}=2.0$ and $2.5$, which introduce a marginal degradation. 
These results indicate that a moderate tube radius provides a good balance between robustness to annotation and prediction noise and sufficient geometric discrimination, and that the 3D-TLIoU loss consistently improves 3D lane fitting quality without requiring fine-tuning of this hyperparameter.
